# Supplementary material for: OmniSDF: Scene Reconstruction using Omnidirectional Signed Distance Functions and Adaptive Binoctrees
Source: arXiv:2404.00678 source file (2024-03-31)
Supplement: Supplementary file 1 [file spherical-3d-recon-supple.tex]

%\documentclass[10pt,twocolumn,letterpaper]{article}
\documentclass[spherical-3d-recon-supple.tex]{subfiles}
\usepackage{cvpr}              %

\input{mypackages}

\definecolor{cvprblue}{rgb}{0.21,0.49,0.74}
\usepackage[pagebackref,breaklinks,colorlinks,citecolor=cvprblue]{hyperref}

\def\paperID{3029} %
\def\confName{CVPR}
\def\confYear{2024}

\input{title}

\input{authors}

\begin{document}
	\clearpage
	\setcounter{page}{1}
	\maketitlesupplementary
	
	\input{sec/supple3}

\begingroup
\raggedright
\small
\def\addvspace#1{\vspace{4pt}}
{
    \small
    \bibliographystyle{ieeenat_fullname}
    \bibliography{spherical-3d-recon}
}
\endgroup 


\end{document}
